# Supplementary material for: ShapeCrafter: A Recursive Text-Conditioned 3D Shape Generation Model
Source: arXiv:2207.09446 source file (2023-04-08)
Supplement: Supplementary file 1 [file supplementary.tex]

\documentclass{article}

% if you need to pass options to natbib, use, e.g.:
%     \PassOptionsToPackage{numbers, compress}{natbib}
% before loading neurips_2022

% ready for submission
% \usepackage[preprint]{neurips_2022}

% to compile a preprint version, e.g., for submission to arXiv, add add the
% [preprint] option:
%     \usepackage[preprint]{neurips_2022}

% to compile a camera-ready version, add the [final] option, e.g.:
%     \usepackage[final]{neurips_2022}

\usepackage[final,nonatbib]{neurips_2022}

\usepackage[utf8]{inputenc} % allow utf-8 input
\usepackage[T1]{fontenc}    % use 8-bit T1 fonts
\usepackage{hyperref}       % hyperlinks
\usepackage{url}            % simple URL typesetting
\usepackage{booktabs}       % professional-quality tables
\usepackage{amsfonts}       % blackboard math symbols
\usepackage{nicefrac}       % compact symbols for 1/2, etc.
\usepackage{microtype}      % microtypography
\usepackage{xcolor}         % colors
\usepackage{graphicx}
\usepackage{array}
\input{macros}
\usepackage{subcaption}

\newcommand{\modelname}{ShapeCrafter\xspace}

% \title{Text-conditioned Shape Generation with Recursive Generation Model}
\title{\modelname: A Recursive Text-Conditioned 3D Shape Generation Model}
% \title{\methodname: Recursive Text-Conditioned 3D Shape Generation}
% \title{\methodname: Text-Conditioned Recursive\\Crafting of 3D Shapes}
% \title{\methodname: Recursive Text-Conditioned\\Crafting of 3D Shapes}
% \title{\methodname: Recursive Text-Conditioned\\Generation of 3D Shapes}
% \title{\methodname: Recursive Text-Conditioned Generation and Evolution of 3D Shapes}

% The \author macro works with any number of authors. There are two commands
% used to separate the names and addresses of multiple authors: \And and \AND.

% Using \And between authors leaves it to LaTeX to determine where to break the
% lines. Using \AND forces a line break at that point. So, if LaTeX puts 3 of 4
% authors names on the first line, and the last on the second line, try using
% \AND instead of \And before the third author name.

\begin{document}

\maketitle
\vspace{-2cm}
\begin{center}
    \Large{\textbf{Supplementary Document}}
\end{center}

\input{supp/text/00_Intro}
\input{supp/text/02_RealTimeDemo}
\input{supp/text/01_Experiment}
\input{supp/text/00_Visualization}
\input{supp/text/04_Limitation}
\input{supp/text/05_Network}

%%%%%%%%%%%%%%%%%%%%%%%%%%%%%%%%%%%%%%%%%%%%%%%%%%%%%%%%%%%%
% \appendix

\newpage
\bibliography{ref} 
\bibliographystyle{plain}

\end{document}
